# Supplementary material for: Rigid Body Dynamic Simulation with Line and Surface Contact
Source: arXiv:2010.02291 source file (2020-10-07)
Supplement: Supplementary file 1 [file appendix.tex]

\section*{Appendix}
\subsection{Normal cone}
As shown in Figure~\ref{figure:contact_nonpenetration_multiple}, when objects are described by intersection of convex functions, there can be contact points lying at the intersection of multiple functions (vertices and points on edges). The normals at these points are not uniquely defined. For any point $\bm{x}$ that lies at intersection of multiple functions, say $f_i(\bm{x}) = 0$, where $i$ belongs to an index set $II$, we can define a normal cone, $\mathcal{C}(\bm{F},\bm{x})$, that consists of all vectors in the conic hull of the normals for each function of object $F$ at $\bm{x}$:
$$\mathcal{C}(\bm{F},\bm{x}) = \{ \bm{y} \vert  \bm{y} = \sum_{i \in II} \beta_i \nabla f_i(\bm{x}), \beta_i\ge 0\}$$
where $\beta_i$ are non-negative constants.
%Now we can define $\mathcal{C}(\bm{F},\bm{a}_1)$ as the normal cone at ECP $\bm{a}_1$ for object $F$, and define $\mathcal{C}(\bm{G},\bm{a}_2)$ as the normal cone at ECP $\bm{a}_2$ for object $G$.
Note that:
\begin{enumerate}
\item For surface contact, the normal cone of any point can lie in the  interior or on the boundary of the contact surface. As shown in the figure~\ref{figure:contact_nonpenetration_c}, when in the {\color{red} relative} interior of the surface, the cone 
contains one function of the plane for contact surface and the cone can be written as a normal vector of the contact surface. When on the boundary, although the cone contains multiple functions, it must include the function of the contact surface. Because the curvature of the flat surface is zero, thus we can define one equivalent normal vector for the contact points on surface. 
\item For line contact, the normal cone of any point can lie in the interior  or on the end points of contact line segment. As shown in the figure~\ref{figure:contact_nonpenetration_b} and~\ref{figure:contact_nonpenetration_e}, when in the interior of the line segment, the contact region is the intersection of two surfaces of the object and the cone is the conic combination of the normal vectors of these two surface functions. When on the endpoints of the line segment, the end points are defined by the intersection of multiple surfaces which includes the same two surfaces of the interior case. Thus normal cone of the endpoints must contain the same two functions of surfaces as in the interior case. Because the curvature along this line segment is zero, we can define one equivalent normal cone for the line segment.
\item The normal cone for the line or surface also defines the set of supporting hyperplanes to the line or surface~\cite{rockafellar1970convex}.
\end{enumerate}
\subsection{Separating hyperplane theorem}
The separating hyperplane theorem states that two nonempty convex sets in $\mathbb{R}^n$ can be properly separated by a hyperplane if and only if their interiors are disjoint~\cite{rockafellar1970convex}. When object are separate, the normal to the separating hyperplane is along the line joining the closest points on the two sets. When two sets have line or surface contact without intersection, a separating hyperplane is also a supporting hyperplane for the contact line or surface on both the sets. Thus, in this case, the separating hyperplane theorem implies that: two non-empty convex objects can have a common supporting hyperplane for the contact line or surface on both sets if and only if their interiors are disjoint. To sum up:

%When objects are separate, the normal to a separating hyperplane is along the line joining the ECPs on the two objects. When objects have line or surface contact with each other without intersection, a separating hyper plane is also a supporting hyperplane which is defined by ECP $\bm{a}_1$ or $\bm{a}_2$ for both objects (ECP $\bm{a}_1$ or $\bm{a}_2$ is a point on the contact line or surface). Because any point on a contact line or surface defines the same normal cone, so the entire contact line or surface has the same set of supporting hyperplanes. Thus, in this case, the separating hyperplane theorem implies that: two non-empty convex objects can have a common supporting hyperplane on the contact line or surface of both sets if and only if their interiors are disjoint. 
\begin{enumerate}
\item When the distance between two objects $F$ and $G$ is greater than zero and ECPs $\bm{a}_1$ and $\bm{a}_2$ on $F$ and $G$ are the closest points on the boundary of two convex objects, the vector $\bm{a}_2 - \bm{a}_1$ lies within the set $\mathcal{C}(\bm{F},\bm{a}_1)$ and also within the set $-\mathcal{C}(\bm{G},\bm{a}_2)$, thus $\mathcal{C}(\bm{F},\bm{a}_1) \cap -\mathcal{C}(\bm{G},\bm{a}_2) \neq \emptyset$.

\item When two objects' distance is zero and have line or surface contact without intersection, set $\mathcal{C}(\bm{F},\bm{a}_1)$ and set $\mathcal{C}(\bm{G},\bm{a}_2)$ defines the set of supporting hyperplanes for contact line or surface on $F$ and $G$. Thus $\mathcal{C}(\bm{F},\bm{a}_1) \cap \mathcal{C}(\bm{G},\bm{a}_2) \neq \emptyset$.

\item If the distance is zero and the two objects intersect, then $\mathcal{C}(\bm{F},\bm{a}_1) \cap \mathcal{C}(\bm{G},\bm{a}_2) = \emptyset$, which implies that there is no hyperplane that can separate the two objects.
\end{enumerate}
